# Supplementary material for: Instanton counting with a surface operator and the chain-saw quiver
Source: arXiv:1105.0357 ancillary file (2011-07-16)
Supplement: Supplementary file 1 [file w2m1n.pdf]

The code is hereby open-sourced; if you use it in your research, please acknowledge it in the paper.

```
If[$VersionNumber < 8,
  << Combinatorica`; Unprotect[Combinatorica`V]; Clear[Combinatorica`V] ]
```

---

## Instanton calculation for general surface operator.

$Y$  is the label of the fixed point, given by Young diagrams arranged in the form of the Young diagram labeling the surface operator. When the surface operator is of type (2,1), an example is  $Y = \{\{\{1,1\}, \{3,2,1\}\}, \{\{4\}\}\}$ .  $A$  is the equivariant parameter for  $U(N)$ , again arranged in the form of the Young diagram labeling the surface operator. For example,  $A = \{\{a_1, A_1\}, \{a_2\}\}$ .

```
depth[Y_] := Max @@ Length /@ Flatten[Y, 1]

appendZero[YY_] :=
  With[{d = depth[YY]}, Table[Table[Table[If[1 ≤ Length[YY[[i, j]]], YY[[i, j, 1]], 0], {1, 1, d}],
    {j, 1, Length[YY[[i]]}], {i, 1, Length[YY]}]]

head[A_, I_, s_] := Module[{n = Length[A]}, Exp[-(I / n)  $\epsilon_2$  + A[[I, s]]]

WW[A, I] is the character of  $W_I$ , and VV[A, Y, I] is the character of  $V_I$  in the paper.

WW[A_, I_] := Sum[head[A, I, s], {s, 1, type[I]}]

VV[A_, YY_, I_] := Module[{Y = appendZero[YY], n = Length[YY], type = Length /@ YY},
  Sum[Module[{X = Mod[I + 1 - J, n, 1]}, Sum[ Sum[
    head[A, X, s] Exp[(1 - J)  $\epsilon_2$  / n] Exp[(1 - j)  $\epsilon_1$ ]
    , {j, 1, Y[[X, s, J]]}
    , {s, 1, type[X]}]]
    , {J, 1, depth[Y]}]]

CONJ[x_] := x /. Exp[w_] => Exp[-w]
```

The character of the tangent space at the fixed point labeled by  $Y$ .

```
char[A_, YY_] := Module[{n = Length[A]}, Sum[Module[{J = If[I == 1, n, I - 1]},
  -(1 - Exp[ $\epsilon_1$ ]) CONJ[VV[A, YY, I]] VV[A, YY, I] +
  (1 - Exp[ $\epsilon_1$ ]) Exp[ $\epsilon_2$  / n] CONJ[VV[A, YY, J]] VV[A, YY, I]
  + CONJ[WW[A, I]] VV[A, YY, I]
  + Exp[ $\epsilon_1$  +  $\epsilon_2$  / n] CONJ[VV[A, YY, J]] WW[A, I] ], {I, 1, n}]]
```

And the code to convert the character to the fixed point contribution.

```
weight[YY_] := Module[{Y = appendZero[YY], n = Length[YY], type = Length /@ YY},
  Product[xi ^ Sum[Sum[Y[[Mod[i - 1 + 1, n, 1], ii, 1]], {ii, 1, type[Mod[i - 1 + 1, n, 1]]}],
    {1, 1, depth[Y]}], {i, 1, n}]]

eigenlist[0] := {}

eigenlist[a_?IntegerQ Exp[b_]] := Table[b, {i, 1, a}]

eigenlist[ Exp[b_]] := {b}

eigenlist[x_ + y_] := eigenlist[x] ~Join~ eigenlist[y]

denom[A_, YY_] := 1 / (Times @@ eigenlist[ char[A, YY] // Expand])
```

The code to generate the fixed points of a surface operator, given the total number of boxes.

```
YoungTuples[1, tot_] := {#} & /@ IntegerPartitions[tot]

YoungTuples[n_, tot_] :=
  YoungTuples[n, tot] = Flatten[Table[Flatten[ Outer[Prepend[#2, #1] &,
    IntegerPartitions[r], YoungTuples[n - 1, tot - r], 1, 1], 1], {r, 0, tot}], 1]
```

```

youngyoung[type_, Y_] :=
  Block[{t = Table[Module[{x = Sum[type[[1]], {1, 1, i - 1}], Table[j, {j, x + 1, x + type[[i]]}],
    {i, 1, Length[type]}]}, Map[Y[[#]] &, t, {2}]]
generalFP[type_, tot_] := youngyoung[ type, #] & /@ YoungTuples[Plus @@ type, tot]

```

## W-algebras.

### ■ Setting up the current algebra

W-algebra of type  $2^m 1^n$  will be realized in the  $U(m+n) \times U(n)$  current algebra. J is for  $U(m+n)$  and JJ is for  $U(n)$ .

Commutator of modes. The level of the non - Abelian current X is given by level[X]

```

com[J_[a_, b_, n_], J_[c_, d_, m_]] := -If[b == c, J[a, d, n + m], 0] +
  If[a == d, J[c, b, n + m], 0] + If[a == d && b == c && n + m == 0, n level[J] Id[], 0]

```

It's important that  $U(1)$  parts of  $U(m+n)$  and  $U(n)$  have off-diagonal components in their level,  $J[a,b](z) JJ[c,d](w) \sim \delta^a_b \delta^c_d / (z-w)^2 \dots$ . This was the last piece I was missing to make this program work! They are explicitly put here.

```

com[J[a_, a_, n_], JJ[c_, c_, m_]] := -n KroneckerDelta[n, -m] Id[]

```

```

com[JJ[a_, a_, n_], J[c_, c_, m_]] := -n KroneckerDelta[n, -m] Id[]

```

```

com[_, _] := 0

```

Commutator of general elements.

```

COM[x_, y_] := x ** y - y ** x

```

Implementation of the Verma module. The basis vectors are denoted by  $Q[ \dots ]$  where  $\dots$  are either modes of J or JJ, or ket[] or bra[] to mark the end of an expression.

```

alg = Id[] | J[_, _, _] | JJ[_, _, _];

```

```

algQ[x_] := MatchQ[x, alg]

```

```

listize[x_] := {#, Coefficient[x, #]} & /@ Union[ Cases[x // Expand, alg, {0, Infinity}]]

```

```

comlist[a_, b_] := listize[com[a, b]]

```

Modes inside  $Q[ \dots ]$  are automatically interchanged so that they have a standard ordering defined by  $o[ \dots ]$ .

```

cartanQ[J_[a_, b_, n_]] := a == b && n == 0

```

```

annQ[J_[a_, b_, n_]] := n > 0 || (n == 0 && a > b)

```

```

creQ[J_[a_, b_, n_]] := n < 0 || (n == 0 && a < b)

```

```

o[J[a_, b_, n_]] := 10 000 n + (a - b) + a / 100

```

```

o[JJ[a_, b_, n_]] := 10 000 n + (a - b) + a / 100 + 1 / 1000

```

```

o[ket[]] := 1 000 000 000

```

```

o[bra[]] := -1 000 000 000

```

```

Q[a___, Id[], b___] := Q[a, b]

```

```

Q[x___, a_, ket[]] /; annQ[a] := 0

```

```

Q[x___, a_, ket[]] /; cartanQ[a] := value[a] Q[x, ket[]]

```

```

Q[bra[], a_, x___] /; creQ[a] := 0

```

```

Q[bra[], a_, x___] /; cartanQ[a] := value[a] Q[bra[], x]

```

```

Q[bra[], ket[]] := 1

```

```
Q[x____, a_, b_, y____] /; o[a] > o[b] :=
  (Plus@@ (#[[2]] Q[x, #[[1]], y] & /@ comlist[a, b])) + Q[x, b, a, y]
```

Rules for the product of modes outside of Q. Somehow it was important to apply commutation relation only inside Q. Otherwise *Mathematica* often went down to infinite loop...

```
Unprotect[NonCommutativeMultiply];

NonCommutativeMultiply /: op_ ** Q[x____] /; algQ[op] := Q[op, x]
NonCommutativeMultiply /: Q[x____] ** op_ /; algQ[op] := Q[x, op]
NonCommutativeMultiply /: (a_ + b_) ** c_ := a ** c + b ** c
NonCommutativeMultiply /: a_ ** (b_ + c_) := a ** b + a ** c
NonCommutativeMultiply /: a_ ** (b_ Q[x____]) := b (a ** Q[x])
NonCommutativeMultiply /: (b_ Q[x____]) ** a_ := b (Q[x] ** a)
NonCommutativeMultiply /: (a_ b_) ** c_ /; FreeQ[a, Q] := a (b ** c)
NonCommutativeMultiply /: a_ ** (b_ c_) /; FreeQ[b, Q] := b (a ** c)
NonCommutativeMultiply /: Q[x____] ** Q[y____] := Q[x, y]
NonCommutativeMultiply /: a_ ** 0 := 0
NonCommutativeMultiply /: 0 ** a_ := 0
NonCommutativeMultiply /: a_ ** Id[] /; algQ[a] := a
NonCommutativeMultiply /: Id[] ** a_ /; algQ[a] := a
Protect[NonCommutativeMultiply];
```

Normal ordering and partial derivative of currents. This is the OPE normal ordering, not the more naive one. Note also that I assumed the dimension of J is one. Beware if you/I reuse the code in the future for more complicated algebras.

```
normalorderX[J_[a_, b_, n_], j_[c_, d_, m_]] :=
  If[n ≥ 0, j[c, d, m] ** J[a, b, n], J[a, b, n] ** j[c, d, m]]
normalorder[J_[a_, b_, n_], j_[c_, d_, m_]] :=
  Module[{x}, Sum[normalorderX[J[a, b, x], j[c, d, n - x]], {x, -7, 7}]]
partial[J_[a_, b_, n_]] := -(1 + n) J[a, b, n]
```

## ■ Generating states in the current algebra Verma module

Generates all the basis vectors in the Verma module, given the grade/charge. First, we generate the states with number of boxes less than a given number.

```
Js[N_, grade_] :=
  Flatten[Table[J[i, Mod[i + j, N, 1], -Quotient[i + j - 1, N]], {i, 1, N}, {j, 1, grade}], 1]
JJJs[N_, indset_, grade_] := Select[Js[N, grade],
  MatchQ[#, J[a_, b_, _] /; MemberQ[indset, a] && MemberQ[indset, b]] &] /. J → JJ
creators[N_, indset_, grade_] := creators[N, indset, grade] =
  Sort[Js[N, grade] ~Join~ JJJs[N, indset, grade], (o[#1] < o[#2]) &]
states[N_, indset_, grade_] := statesFrom[N, grade, creators[N, indset, grade]]

statesFrom[N_, 0, _] := {Q[ket[]]}
statesFrom[N_, grade_, _] /; grade < 0 := {}
statesFrom[N_, grade_, {}] /; grade > 0 := {}

statesFrom[N_, grade_, {J_[a_, b_, n_], x____}] := statesFrom[N, grade, {J[a, b, n], x}] =
  ((Prepend[#, J[a, b, n]] &) /@ statesFrom[N, grade - (b - n N - a), {J[a, b, n], x}]) ~
  Join~statesFrom[N, grade, {x}]
```

Then we filter them according to the charges.

```
charge[N_, J_[a_, b_, n_]] := Module[{k}, Product[xMod[k, N, 1], {k, a, b - N n - 1}]]
charge[N_, ket[]] := 1
chargeOfQ[N_, Q[x___]] := Times@@ (charge[N, #] & /@ {x})
maxi[q_] := Block[{m = Max[Cases[q, xy → y, {0, Infinity}]]}, If[m ≥ 1, m, 0]]
boxes[q_] := Sum[D[q, xi] /. {x- → 1}, {i, 1, maxi[q]}]
sensibleQ[q_] := And @@ ((# ≥ 0) & /@ Table[D[q, xi] /. {x- → 1}, {i, 1, maxi[q]}])
statesOfCharge[N_, indexset_, q_] := statesOfCharge[N, indexset, q] =
  If[sensibleQ[q], Select[states[N, indexset, boxes[q]], chargeOfQ[N, #] == q &], {}]
braize[Q[x___]] := (Q@@ Sort[daggerE /@ {x}, (o[#1] < o[#2]) &])
daggerE[ket[]] := bra[]
daggerE[J_[a_, b_, n_]] := J[b, a, -n]
brasOfCharge[NN_, indexset_, q_] :=
  brasOfCharge[NN, indexset, q] = braize /@ statesOfCharge[NN, indexset, q]
vars[x_] := Table[ci, {i, 1, Length[x]}]
```

For a vector  $X$  in a Verma module,  $\text{eqn}[x]$  gives the equation  $x=0$  in components so that *Mathematica* can later solve it.

```
eqn[x_] := Block[{basis = Union[Cases[x, Q[___], {0, Infinity}]]},
  If[basis == {}, {}, Module[{dummies = Table[di, {i, 1, Length[basis]}]},
    dummyTable = Table[basis[[i]] → di, {i, 1, Length[basis]}]],
    Table[D[x /. dummyTable, di] == 0, {i, 1, Length[basis]}]]]]
eqn[x_, y_] := eqn[x] ~Join~ eqn[y]
```

## ■ Setting up the Miura transformation

As an input, you need to set the type of the surface operator below.  $NN$  is the number of columns, and  $\text{indexset}$  is the set of columns of height 2

```
NN := Length[type]
indexset := Flatten[Position[type, 2, 1]]
kets[q_] := statesOfCharge[NN, indexset, q]
bras[q_] := brasOfCharge[NN, indexset, q]
dualindexset := Select[Table[i, {i, 1, NN}], ! MemberQ[indexset, #] &];
mm := Length[indexset];
nn := NN - mm;
hi and Hi are the Cartan eigenvalues of U(n+m) and U(m), respectively.
value[J[i_, i_, 0]] := hi
value[JJ[i_, i_, 0]] := Hi
level[J] := kk + mm;
level[JJ] := kk + mm + nn;
diagonal[n_] := Sum[J[a, a, n], {a, 1, NN}] + (Plus @@ (JJ[#, #, n] & /@ indexset))
```

These are the  $W$  generators.  $\text{jj}[a,b]$  are  $U(m)$  currents,  $\text{J}[i,j]$  are  $U(n)$  currents,  $U$  and  $U_t$  (which stands for  $U$  tilde) are the bifundamentals,  $\text{S}[a,b]$  are cousins of the energy momentum tensor

```

jj[a_, b_, n_] := J[a, b, n] + JJ[a, b, n]
U[a_, i_, n_] := J[a, i, n]
Ut[i_, b_, n_] := (Plus @@ (normalorder[JJ[#, b], J[i, #], n] &) /@ indexset)) -
  (Plus @@ (normalorder[J[i, #], J[#, b], n] &) /@ dualindexset)) -
  (kk + NN) partial[J[i, b], n]
S[a_, b_, n_] := - (Plus @@ (normalorder[J[a, #], J[#, b], n] &) /@ dualindexset)) +
  (Plus @@ (normalorder[JJ[#, b], J[a, #], n] &) /@ indexset)) -
  (kk + NN) (1 / 2) (partial[J[a, b], n] - partial[JJ[a, b], n])

```

## Comparisons

```
ra := Random[Integer, {-500, 500}];
```

Shorthand to generate all the fixed points given NN and indexset i.e. the type of partition including the ordering

```
FPS[q_] := Select[generalFP[type, boxes[q]], weight[#] == q &]
```

### ■ 3 = 2 + 1

```
type = {2, 1};
```

V is the Whittaker ket, W is the Whittaker bra. Note that we can't just take the adjoint (in terms of J and JJ) to get W from V, because we need to make Ut the adjoint of U. I decided to compute the two separately.

$x_1$  is the factor counting the fractional instanton for the 1st column,  $x_2$  is the one for the 2nd column, etc.

```
Clear[V, W]; V[1] = Q[ket[]]; W[1] = Q[bra[]]; norm[q_] := W[q] ** V[q];
```

```
W[q_] := W[q] =
  If[! sensibleQ[q], 0, Module[{s = bras[q], w = vars[s].s; soln = Solve[ eqn[
    w ** U[1, 2, 0] - W[q / x1],
    w ** Ut[2, 1, -1] + W[q / x2],
    w ** jj[1, 1, -1],
    w ** S[1, 1, -1],
    w ** J[2, 2, -1]
  ], vars[s]]; If[Length[soln] == 1, W[q] = w /. soln[[1]], Print["can't solve"]]]]
```

```
V[q_] :=
  If[! sensibleQ[q], 0, Module[{s = kets[q], w = vars[s].s; soln = Solve[ eqn[
    Ut[2, 1, 0] ** w - V[q / x1],
    U[1, 2, 1] ** w - V[q / x2],
    jj[1, 1, 1] ** w,
    S[1, 1, 1] ** w,
    J[2, 2, 1] ** w
  ], vars[s]]; If[Length[soln] == 1, V[q] = w /. soln[[1]], Print["can't solve"]]]]
```

Instanton calculation. Each fixed point is labeled by three Young diagrams, arranged in the Young diagram of the form 2+1

```
inst[q_] := Plus @@ (denom[{a1, A1}, {a2}], #] & /@ FPS[q])
```

For a column of height two, we assign the equivariant parameters {a, A}; for a column of height one, just {a}.

h is the eigenvalue of the Cartan of U(m+n), H is for U(m)

```
rule = {ε1 → 1, a1 → h1, a2 → h2 - 1, A1 → H1 + kk + 1, ε2 → -kk - 3};
```

```
norm[x1]
```

$$-\frac{1}{(h_1 - h_2) (-1 - kk + h_2 - H_1)}$$

```

inst[x1] /. rule


$$\frac{1}{(-h_1 + h_2)(-1 - kk + h_1 - H_1)} + \frac{1}{(-1 - kk + h_2 - H_1)(1 + kk - h_1 + H_1)}$$

% - %% // Simplify
0

norm[x1 x2] // Simplify


$$\frac{\left( -(1 + kk) h_1^2 + 2 h_2^2 - 2 h_2 H_1 - (1 + kk) H_1 (3 + 2 kk + H_1) + h_1 (3 + 5 kk + 2 kk^2 - 2 h_2 + 2 (2 + kk) H_1) \right)}{(3 + kk)(h_1 - h_2)(1 + kk - h_1 + h_2)(1 + h_1 - H_1)(h_2 - H_1)(3 + 2 kk - h_1 + H_1)(1 + kk - h_2 + H_1)}$$

inst[x1 x2] /. rule // Simplify


$$\frac{\left( -(1 + kk) h_1^2 + 2 h_2^2 - 2 h_2 H_1 - (1 + kk) H_1 (3 + 2 kk + H_1) + h_1 (3 + 5 kk + 2 kk^2 - 2 h_2 + 2 (2 + kk) H_1) \right)}{(3 + kk)(h_1 - h_2)(1 + kk - h_1 + h_2)(1 + h_1 - H_1)(h_2 - H_1)(3 + 2 kk - h_1 + H_1)(1 + kk - h_2 + H_1)}$$

% - %% // Simplify
0

h1 = ra; h2 = ra; H1 = ra; kk = ra;

norm[x1 ^ 2 x2 ^ 2]


$$\frac{216\,752\,586\,706\,913\,119\,896\,629}{437\,292\,243\,853\,195\,865\,317\,624\,783\,131\,003\,422\,208\,000}$$

inst[x1 ^ 2 x2 ^ 2] /. rule


$$\frac{216\,752\,586\,706\,913\,119\,896\,629}{437\,292\,243\,853\,195\,865\,317\,624\,783\,131\,003\,422\,208\,000}$$

% - %%
0

There are this numeber of states in the Verma module ...

kets[x1 ^ 2 x2 ^ 2] // Length
15

while there are this number of fixed points at this degree...

FPs[x1 ^ 2 x2 ^ 2] // Length
22

h1 = .; h2 = .; H1 = .; kk = .;

■ 6 = 2 + 2 + 1 + 1
type = {2, 2, 1, 1};

The Whittaker ket and bra.

Clear[V, W]; V[1] = Q[ket[]]; W[1] = Q[bra[]]; norm[q_] := W[q] ** V[q];

```

```

W[q_] := W[q] =
  If[! sensibleQ[q], 0, Module[{s = bras[q], w, soln}, w = vars[s].s; soln = Solve[ eqn[
    w**S[1, 2, 0] - W[q/x1],
    w**jj[1, 2, 0],
    w**U[2, 3, 0] - W[q/x2],
    w**J[3, 4, 0] + W[q/x3],
    w**Ut[4, 1, -1] + W[q/x4],
    w**diagonal[-1]
  ], vars[s]]; If[Length[soln] == 1, W[q] = w /. soln[[1]], Print["can't solve"]]]]

V[q_] :=
  If[! sensibleQ[q], 0, Module[{s = kets[q], w, soln}, w = vars[s].s; soln = Solve[ eqn[
    s[2, 1, 0]**w - V[q/x1],
    jj[2, 1, 0]**w,
    Ut[3, 2, 0]**w - V[q/x2],
    J[4, 3, 0]**w - V[q/x3],
    U[1, 4, 1]**w - V[q/x4],
    diagonal[1]**w
  ], vars[s]]; If[Length[soln] == 1, V[q] = w /. soln[[1]], Print["can't solve"]]]]

```

For a column of height two, we assign the equivariant parameters {a, A}; for a column of height one, just {a}.

h is the eigenvalue of the Cartan of U(m+n), H is for U(m)

```
inst[q_] := Plus @@ (denom[{a1, A1}, {a2, A2}, {a3}, {a4}], #] & /@ FPS[q])
```

```
rule = {e1 -> 1, a1 -> h1, a2 -> h2 - 1, a3 -> h3 - 2,
  a4 -> h4 - 3, A1 -> H1 + kk + 2, A2 -> H2 + kk + 1, e2 -> -kk - 6};
```

```
inst[x1] /. rule // Simplify
```

$$\frac{h_1 - h_2 + H_1 - H_2}{(h_1 - h_2) (2 + kk - h_2 + H_1) (H_1 - H_2) (2 + kk - h_1 + H_2)}$$

```
norm[x1] // Simplify
```

$$\frac{h_1 - h_2 + H_1 - H_2}{(h_1 - h_2) (2 + kk - h_2 + H_1) (H_1 - H_2) (2 + kk - h_1 + H_2)}$$

```
% - %% // Simplify
```

```
0
```

```
h1 = ra; h2 = ra; h3 = ra; h4 = ra; H1 = ra; H2 = ra; kk = ra;
```

```
inst[x1 x2 x3 x4] /. rule
```

```
38 985 782 483 041 034 455 076 820 241 104 196 337 /
96 906 713 715 484 780 326 653 737 202 547 506 580 629 530 983 360 000 000
```

```
norm[x1 x2 x3 x4]
```

```
38 985 782 483 041 034 455 076 820 241 104 196 337 /
96 906 713 715 484 780 326 653 737 202 547 506 580 629 530 983 360 000 000
```

There are this number of states in the Verma module ...

```
kets[x1 x2 x3 x4] // Length
```

```
23
```

while there are this number of fixed points at this degree...

```
FPS[x1 x2 x3 x4] // Length
```

```
35
```

```
h1 = .; h2 = .; h3 = .; h4 = .; H1 = .; H2 = .; kk = .;
```

■  $6 = 2 + 1 + 2 + 1$

```

type = {2, 1, 2, 1};

Clear[V, W]; V[1] = Q[ket[]]; W[1] = Q[bra[]]; norm[q_] := W[q] ** V[q]

W[q_] := W[q] =
  If[! sensibleQ[q], 0, Module[{s = bras[q], w, soln}, w = vars[s].s; soln = Solve[ eqn[
    w ** U[1, 2, 0] - W[q / x1],
    w ** Ut[2, 3, 0] + W[q / x2],
    w ** jj[1, 3, 0],
    w ** S[1, 3, 0],
    w ** U[3, 4, 0] - W[q / x3],
    w ** Ut[4, 1, -1] + W[q / x4],
    w ** jj[3, 1, -1],
    w ** S[3, 1, -1],
    w ** diagonal[-1]
  ], vars[s]]; If[Length[soln] == 1, W[q] = w /. soln[[1]], Print["can't solve"]]]]

V[q_] :=
  If[! sensibleQ[q], 0, Module[{s = kets[q], w, soln}, w = vars[s].s; soln = Solve[ eqn[
    Ut[2, 1, 0] ** w - V[q / x1],
    U[3, 2, 0] ** w - V[q / x2],
    jj[3, 1, 0] ** w,
    S[3, 1, 0] ** w,
    Ut[4, 3, 0] ** w - V[q / x3],
    U[1, 4, 1] ** w - V[q / x4],
    jj[1, 3, 1] ** w,
    S[1, 3, 1] ** w,
    diagonal[1] ** w
  ], vars[s]]; If[Length[soln] == 1, V[q] = w /. soln[[1]], Print["can't solve"]]]]

inst[q_] := Plus @@ (denom[{a1, A1}, {a2}, {a3, A3}, {a4}], #] & /@ FPS[q])

rule = {e1 → 1, a1 → h1, a2 → h2 - 1, a3 → h3 - 2,
  a4 → h4 - 3, A1 → H1 + kk + 2, A3 → H3 + kk + 1, e2 → -kk - 6};

inst[x1] /. rule // Simplify


$$\frac{1}{(h_1 - h_2) (2 + kk - h_2 + H_1)}$$

norm[x1] // Simplify


$$\frac{1}{(h_1 - h_2) (2 + kk - h_2 + H_1)}$$

% - %% // Simplify

0

inst[x4] /. rule // Simplify


$$\frac{1}{(2 + kk - h_1 + h_4) (h_4 - H_1)}$$

norm[x4] // Simplify


$$\frac{1}{(2 + kk - h_1 + h_4) (h_4 - H_1)}$$

% - %% // Simplify

0

h1 = ra; h2 = ra; h3 = ra; h4 = ra; H1 = ra; H3 = ra; kk = ra;

```



```
inst[x1 ^ 2 x2 x3 ^ 2 x4] /. rule
```

```
152 026 623 163 681 205 822 020 709 111 553 780 407 012 561 143 /
17 607 048 863 974 674 772 237 586 632 398 217 331 901 561 594 916 305 598 172 107 247 512 800 000
```

```
norm[x1 ^ 2 x2 x3 ^ 2 x4]
```

```
152 026 623 163 681 205 822 020 709 111 553 780 407 012 561 143 /
17 607 048 863 974 674 772 237 586 632 398 217 331 901 561 594 916 305 598 172 107 247 512 800 000
```

There are this number of states in the Verma module ...

```
kets[x1 ^ 2 x2 x3 ^ 2 x4] // Length
```

```
35
```

while there are this number of fixed points at this degree...

```
FPS[x1 ^ 2 x2 x3 ^ 2 x4] // Length
```

```
165
```

```
h1 = .; h2 = .; h3 = .; h4 = .; H1 = .; H3 = .; kk = .;
```

■ **6 = 2 + 2 + 2**

```
type = {2, 2, 2};
```

```
Clear[V, W]; V[1] = Q[ket[]]; W[1] = Q[bra[]]; norm[q_] := W[q] ** V[q]
```

```
W[q_] := W[q] =
```

```
If[! sensibleQ[q], 0, Module[{s = bras[q], w, soln}, w = vars[s].s; soln = Solve[ eqn[
  w ** S[1, 2, 0] - W[q / x1],
  w ** jj[1, 2, 0],
  w ** S[2, 3, 0] - W[q / x2],
  w ** jj[2, 3, 0],
  w ** S[3, 1, -1] - W[q / x3],
  w ** jj[3, 1, -1],
  w ** diagonal[-1]
], vars[s]]; If[Length[soln] == 1, W[q] = w /. soln[[1]], Print["can't solve"]]]]
```

```
V[q_] :=
```

```
If[! sensibleQ[q], 0, Module[{s = kets[q], w, soln}, w = vars[s].s; soln = Solve[ eqn[
  S[2, 1, 0] ** w - V[q / x1],
  jj[2, 1, 0] ** w,
  S[3, 2, 0] ** w - V[q / x2],
  jj[3, 2, 0] ** w,
  S[1, 3, 1] ** w - V[q / x3],
  jj[1, 3, 1] ** w,
  diagonal[1] ** w
], vars[s]]; If[Length[soln] == 1, V[q] = w /. soln[[1]], Print["can't solve"]]]]
```

```
inst[q_] := Plus @@ (denom[{a1, A1}, {a2, A2}, {a3, A3}] , #] & /@ FPS[q])
```

```
rule = {ε1 → 1, a1 → h1, a2 → h2 - 1, a3 → h3 - 2,
  A1 → H1 + kk + 3, A2 → H2 + kk + 2, A3 → H3 + kk + 1, ε2 → -kk - 6};
```

```
h1 = ra; h2 = ra; h3 = ra; H1 = ra; H2 = ra; H3 = ra; kk = ra;
```

```
norm[x1 ^ 2 x2 x3] // Simplify
```

```
1 175 659 574 791 733 778 797 460 257 770 528 465 320 505 021
```

```
6 052 339 853 125 677 217 133 829 586 896 590 167 974 898 531 320 947 559 096 478 556 160 000 000 000
```

```
inst[x1 ^ 2 x2 x3] /. rule // Simplify
```

```
1 175 659 574 791 733 778 797 460 257 770 528 465 320 505 021
```

```
6 052 339 853 125 677 217 133 829 586 896 590 167 974 898 531 320 947 559 096 478 556 160 000 000 000
```

There are this number of states in the Verma module ...

```
kets[x1 ^ 2 x2 x3] // Length
```

```
52
```

while there are this number of fixed points at this degree...

```
FPS[x1 ^ 2 x2 x3] // Length
```

```
52
```

```
h1 = . ; h2 = . ; h3 = . ; H1 = . ; H2 = . ; H3 = . ; kk = . ;
```
